# Supplementary material for: Step-Video-TI2V Technical Report: A State-of-the-Art Text-Driven Image-to-Video Generation Model
Source: arXiv:2503.11251 source file (2025-03-14)
Supplement: Supplementary file 2 [file a2_evalution.tex]

\section{Evalution Details}
\label{sec:appendix:evalution}

\subsection{Math Evalution}
\label{sec:appendix:math_evalution}
We conducted a comprehensive evaluation of the model across various math reasoning benchmarks, encompassing a range of difficulties from elementary to university level, multiple mathematical domains, and diverse question types including multiple-choice and open-ended questions.
Our benchmarks include GSM8k~\citep{cobbe2021gsm8k}, MATH \citep{hendrycks2021measuring}, GSM-Hard \citep{gao2022pal}, SVAMP~\citep{patel2021svamp}, ASDIV \citep{miao-etal-2020-diverse},  MAWPS \citep{koncel-kedziorski-etal-2016-mawps}, TabMWP (TAB) \citep{lu2023dynamic}, MathQA (MQA) \citep{amini2019mathqa}, MMLU-STEM \citep{hendrycks2020measuring}, and SAT~\citep{azerbayev2023llemma}.

\subsection{General Evalution}
\label{sec:appendix:general_evalution}
In the evaluation of general domain, we followed the lm-evaluation-harness~\citep{eval-harness} and evalute model on MMLU~\citep{hendrycks2020measuring}, BBH~\citep{suzgun2022challenging}, AGIEval~\citep{zhong2023agieval}, ARC-Easy and ARC-Challenge~\citep{clark2018arc}, BoolQ~\citep{clark2019boolq}, PIQA~\citep{bisk2020piqa}, Hellaswag~\citep{zellers2019hellaswag}, WinoGrande~\citep{sakaguchi2021winogrande}, OpenBookQA~\citep{mihaylov2018obqa}. 
On HumanEval~\citep{zheng2023codegeex} and TydiQA~\citep{clark2020tydiqa}, we follow the evaluation pipeline of open-instrcut~\citep{ivison2023camels} and report {Pass@1} and {Pass@10} for HumanEval and {F1} for TydiQA. For MBPP~\citep{austin2021mbpp} benchmark, we follow the evaluation pipeline of DeepSeek-Coder~\citep{deepseek-coder}, and report {Pass@1} and {Pass@10}.

% For math QA tasks MATH and GSM8K, we use the same evaluation method as described in \autoref{sec:appendix:math_evalution}.
