# Supplementary material for: Step-Video-TI2V Technical Report: A State-of-the-Art Text-Driven Image-to-Video Generation Model
Source: arXiv:2503.11251 source file (2025-03-14)
Supplement: Supplementary file 3 [file a3_acc_loss.tex]

\section{Relate the Selected Tokens' Loss to Downstream Task Performance}
\label{sec:appendix:acc_loss}

In this section, we declare the details about correlating the loss of selected tokens with the performance of downstream tasks. Concurrent study has explored similar methods to study the impact of scaling laws with the performance of models in downstream tasks~\citep{gadre2024LanguageMS}. Our analysis here differs in that it aims to elucidate the relationship between the decrease/increase in loss for selected/unselected tokens and the model's performance on downstream tasks. 

We use the average accuracy of MATH and GSM8K as the standard for measuring downstream tasks performance of model. Based on the trend of data points in \autoref{fig:acc_loss}, we propose the relationship between the average accuracy of downstream tasks and selected/unselected tokens' loss,

\begin{equation}
Acc(\mathcal{L}) = \log (a * \mathcal{L} + c)
\end{equation}

The parameters $a$ and $c$ are fitted from the data. If the loss of selected tokens $\mathcal{L}_s$ is used for fitting, then $a > 0$. Conversely, if the loss of unselected tokens $\mathcal{L}_{us}$ is used for fitting, then $a < 0$. Therefore, we believe that training the model on selected tokens can effectively improve its performance on downstream tasks, while unselected tokens may have a detrimental effect on the model's performance in downstream tasks.
