# Supplementary material for: Step-Video-TI2V Technical Report: A State-of-the-Art Text-Driven Image-to-Video Generation Model
Source: arXiv:2503.11251 source file (2025-03-14)
Supplement: Supplementary file 4 [file a4_examples_tokens_selected.tex]

\section{Examples of Tokens Selected by \method{}}

\subsection{Token Selected Examples}
\label{sec:appendix:examples_token_selected}

% \begin{figure*}[t]
% \centering
% \includegraphics[width=\textwidth]{figure/token_select_example.pdf}
% \caption{\textbf{Specific examples of selecting tokens during the selective pretraining process of the \model{}.} The tokens marked in \textcolor[RGB]{30,144,255}{blue} represent the actual tokens trained during the training process, while the remaining black tokens are not trained during the training process.}
% \label{fig:token_select_example}
% \end{figure*}

In \autoref{fig:token_select_example}, we present several examples of tokens selected by the \method{} method, with content marked in \textcolor[RGB]{30,144,255}{blue} indicating the tokens actually chosen during the pretraining process.

\subsection{Dynamic Token Selected}
\label{sec:appendix:dynamic_token_selected}

% \begin{figure*}[t]
% \centering
% \includegraphics[width=\textwidth]{figure/example_dynamic_token.pdf}
% \caption{\textbf{An example of dynamic token selection changes during the training process}, which illustrated with five different score levels represented by \textcolor[RGB]{0,0,255}{deep blue}, \textcolor[RGB]{30,144,255}{light blue}, black, \textcolor[RGB]{255,180,150}{light orange}, and \textcolor[RGB]{255,100,0}{dark orange}. The bluer the color indicates a higher tendency for the token to be selected, while the more orange the color suggests a lower tendency for the token to be selected.}
% \label{fig:example_dynamic_token}
% \end{figure*}

In \autoref{fig:example_dynamic_token}, we display the dynamic changes in token selection tendencies throughout the \method{} training process. We chose four checkpoints during the training process (0\%, 33\%, 66\%, and 100\%) to analyze the current tendencies in token selection. The preferences for token selection are indicated by different colors, ranging from high to low preference, typically represented as \textcolor[RGB]{0,0,255}{deep blue}, \textcolor[RGB]{30,144,255}{blue}, black, \textcolor[RGB]{255,180,150}{orange}, and \textcolor[RGB]{255,100,0}{dark orange}, respectively.
