# Supplementary material for: Step-Video-TI2V Technical Report: A State-of-the-Art Text-Driven Image-to-Video Generation Model
Source: arXiv:2503.11251 source file (2025-03-14)
Supplement: Supplementary file 5 [file a5_self-reference_setting.tex]

\section{Self-Reference Setting}
\label{sec:appendix:self-reference-setting}

% \begin{table*}[t]
% \centering
% \setlength{\tabcolsep}{2pt}
% \caption{\textbf{Self-Reference results on the Mistral-7B.}}
% \label{tab:self-ref-7b-owm}
% \resizebox{\linewidth}{!}{
% \begin{tabular}{l|ccc|cccccccc|c}
% \toprule
% \textbf{Model} & \multicolumn{1}{c}{\textbf{\begin{tabular}[c]{@{}c@{}}SLM\\ Strategy\end{tabular}}} & \multicolumn{1}{c}{\textbf{\begin{tabular}[c]{@{}c@{}}Uniq.\\ Toks$^*$\end{tabular}}}& \multicolumn{1}{c|}{\textbf{\begin{tabular}[c]{@{}c@{}}Train\\ Toks\end{tabular}}} & \textbf{GSM8K} & \textbf{MATH} & \textbf{SVAMP} & \textbf{ASDiv} & \textbf{MAWPS} & \textbf{TAB}& \textbf{MQA} & \multicolumn{1}{c|}{\textbf{\begin{tabular}[c]{@{}c@{}}MMLU\\ STEM\end{tabular}}} & \textbf{AVG} \\
% \midrule
% Mistral-CT (RM) & - & 14B & 15B & 42.9 & 22.2 & 68.6 & 71.0 & 86.1 & 45.1 & 47.7 & 52.6 & 54.5 \\
% Mistral-SLM & $\mathcal{L}_{\text{RM}}(x_i)$ & 14B & 13.5B & 45.1 & 21.0 & 67.4 & 71.6 & 87.0 & 45.2 & 48.9 & 53.3 & 54.9 \\
% Mistral-SLM & $\mathcal{H}_{\text{RM}}(x_i)$ & 14B & 13.5B & 47.7 & 22.8 & 67.8 & 72.0 & 87.7 & 54.4 & 50.5 & 52.8 & 57.0 \\
% \bottomrule
% \end{tabular}
% }
% \end{table*}

\begin{table*}[t]
\centering
\small
\setlength{\tabcolsep}{2pt}
\caption{\textbf{Full Self-Reference results on Tinyllama-1.1B.}}
\label{tab:self-ref-1b-slm}
\resizebox{\linewidth}{!}{
\begin{tabular}{c|c|cccccc|c}
\toprule
\multicolumn{1}{c|}{\textbf{\begin{tabular}[c]{@{}c@{}}Score\\ Function\end{tabular}}} & \multicolumn{1}{c|}{\textbf{\begin{tabular}[c]{@{}c@{}}Select\\ Ratio\end{tabular}}} & \textbf{GSM8K} & \textbf{MATH} & \textbf{SVAMP} & \textbf{ASDiv} & \textbf{MAWPS} & \textbf{MQA} & \textbf{AVG} \\
\midrule
- & 100\% & 6.3 & 2.6 & 21.7 & 36.7 & 47.7 & 13.9 & 21.5 \\
\midrule
\multirow{5}{*}{$\mathcal{L}_{\text{RM}}(x_i)$} & 90\% & \textbf{7.4} & 4.4 & \textbf{23.4} & 38.7 & 51.9 & \textbf{14.4} & 23.4 \\
& 80\% & 6.4 & \textbf{4.6} & 23.1 & 39.7 & 52.0 & 14.3 & 23.4 \\
& 70\% & 6.7 & \textbf{4.6} & 23.3 & \textbf{40.0} & \textbf{54.5} & 14.3 & \textbf{23.9} \\
& 60\% & 7.0 & \textbf{4.6} & 22.2 & 38.5 & 52.2 & 13.7 & 23.0 \\
& 50\% & 5.7 & 4.2 & 20.7 & 36.7 & 46.7 & 10.3 & 20.7  \\
\midrule

\multirow{5}{*}{$\mathcal{H}_{\text{RM}}(x_i)$}
& 90\% & 6.7 & 3.0 & 23.7 & 40.3 & 52.3 & 13.1 & 23.2 \\
& 80\% & 6.8 & 3.6 & 22.5 & \textbf{40.6} & \textbf{52.9} & 13.6 & 23.3 \\
& 70\% & \textbf{7.0} & 4.8 & 23.0 & 39.3 & 50.5 & 13.5 & 23.0 \\
& 60\% & 6.5 & 4.8 & \textbf{26.5} & 37.3 & 49.7 & \textbf{15.6} & \textbf{23.4} \\
& 50\% & 4.7 & \textbf{5.8} & 20.9 & 33.8 & 42.5 & 11.1 & 19.8  \\
\midrule

\multirow{5}{*}{$\mathcal{H}_{\text{RM}}(x_i)\cup\mathcal{L}_{\text{RM}}(x_i)$}
& $50\% \cup 70\% (80\%)$& 6.4 & 3.6 & 22.7 & 38.4 & 52.6 & 15.3 & 23.2 \\
& $70\% \cup 60\% (77\%)$& 6.3 & 4.6 & 24.4 & 39.6 & 51.4 & \textbf{16.3} & \textbf{23.8} \\
& $70\% \cup 50\% (75\%)$& 6.9 & 5.6 & 23.2 & \textbf{39.9} & \textbf{52.9} & 12.6 & 23.5 \\
& $60\% \cup 60\% (70\%)$& 6.7 & 5.2 & \textbf{24.7} & 39.2 & 50.6 & 14.6 & 23.5 \\
& $60\% \cup 50\% (68\%)$& 7.1 & 5.8 & 21.7 & 37.3 & 49.6 & 15.3 & 22.8 \\
& $60\% \cup 40\% (65\%)$& \textbf{7.3} & \textbf{6.0} & 23.6 & 36.9 & 48.6 & 13.1 & 22.6 \\
\midrule

\multirow{5}{*}{$\mathcal{H}_{\text{RM}}(x_i)\cap\mathcal{L}_{\text{RM}}(x_i)$} 
& $80\% \cap 90\% (76\%)$& 6.0 & 4.4 & 23.7 & 38.5 & 51.2 & 13.3 & 22.8 \\
& $75\% \cap 75\% (72\%)$& 7.8 & 5.2 & \textbf{24.2} & 39.4 & \textbf{54.9} & 14.7 & 24.4 \\
& $70\% \cap 90\% (68\%)$& 6.8 & 4.6 & 22.2 & 40.3 & 53.0 & 14.8 & 23.6 \\
& $80\% \cap 80\% (67\%)$& \textbf{8.2} & \textbf{6.4} & 21.2 & 39.1 & 53.4 & 15.0 & 23.9 \\
& $70\% \cap 70\% (60\%)$& 7.1 & 5.0 & 23.5 & \textbf{41.2} & 53.8 & \textbf{18.0} & \textbf{24.8} \\
\bottomrule
\end{tabular}
}
\end{table*}

In this section, we will provide a detailed introduction to the reference loss score function and information entropy score function in SLM. Reference loss score function is to directly use the loss of the reference model as the basis for selecting tokens. The higher the token's loss of the reference model, the lower the expectation that the token will be selected. The score $\mathcal{L}_{\text{RM}}(x_i)$ can be directly obtained by referring to \autoref{equ:ref_loss}. Information entropy score function is to select the corresponding token based on the information entropy of the reference model in each token. The information entropy of token $x_i$ can be expressed as:

% \mathcal{H}_{\text{RM}}(x_i) = -\sum_{i=1}^{{V} P(t_i)\log P(t_i),

% \begin{equation}
% \mathcal{H}_{\text{RM}}(x_i) = -\sum_{k=1}^{{V}} P(t_k|x< i)\log P(t_k|x<i),
% \end{equation}

\begin{equation}
\mathcal{H}_{\text{RM}}(x_i) = -\sum_{k=1}^{V} P(t_k|x_{<i}) \log P(t_k|x_{<i}),
\end{equation}

where $t_k$ represents the i-th token in the vocabulary, and $V$ represents the size of the vocabulary. The intuition of this strategy is that the higher the information entropy, the higher the uncertainty of the token in the context. Therefore, we consider that if the language model is still uncertain for certain tokens after pretraining, we do not expect that the language model will learn it during pretraining. In \autoref{tab:self-ref-1b-slm}, we provide more SLM results, including different select ratios and combinations of two score functions, for the convenience of the readers to refer to.
%In \autoref{tab:self-ref-7b-owm}, we have added the results of the self-reference of the 7B model, and it can be seen that the Information Entropy Mask strategy is more stable in improving the 7B model compared to the Reference Loss Mask strategy.
