# Supplementary material for: Step-Video-TI2V Technical Report: A State-of-the-Art Text-Driven Image-to-Video Generation Model
Source: arXiv:2503.11251 source file (2025-03-14)
Supplement: Supplementary file 6 [file a6_weak-to-strong.tex]

\section{Weak-to-Strong Generalization}

%1B Tinyllama as ref -> 7B Llama 
\begin{table*}[t]
\centering
\setlength{\tabcolsep}{2pt}
\caption{\textbf{Weak-to-Strong generalization result on math benchmark.}
}
\label{tab:small-ref-result}
\resizebox{\linewidth}{!}{
\begin{tabular}{lc|ccccccccc|c}
\toprule
\textbf{Model} & \textbf{Train Toks} & \textbf{GSM8K} & \textbf{MATH} & \textbf{SVAMP} & \textbf{ASDiv} & \textbf{MAWPS} & \textbf{TAB}& \textbf{MQA} & \multicolumn{1}{c}{\textbf{\begin{tabular}[c]{@{}c@{}}MMLU\\ STEM\end{tabular}}} & \textbf{SAT} & \textbf{AVG} \\
\midrule
Llama-2-7B-CT & 15B & 28.4 & 13.6 & 50.3 & 62.8 & 79.5 & 37.6 & 34.1 & 41.6 & 43.5 & 43.5 \\
Llama-2-7B-CT w/ 1B RM & 10.5B &  29.8 & 16.0 & 55.5 & 63.7 & 80.4 & 37.9 & 34.3 & 38.2 & 43.8 & 44.4 \\
\bottomrule
\end{tabular}
}
\end{table*}

Apart from the main experiments where we use the same base model for the reference and continual pretraining, we also investigate if a smaller reference model can effectively guide the pretraining of a larger model.
We use Tinyllama-1.1B as reference model and continual pretraining Llama-2-7B on 15B OpenWebMath tokens.
Results presented in \autoref{tab:small-ref-result} indicate that, despite the considerable gap between the small and large models~\citep{contrastivedecoding23}, employing the small reference model to token selection can still yield benefits to the pre-training of the larger model.
If reference and training models have different vocabularies, one can consider performing token alignment \citep{wan2024knowledge, fu2023specializing}, which we leave for future work.
