# Supplementary material for: Step-Video-TI2V Technical Report: A State-of-the-Art Text-Driven Image-to-Video Generation Model
Source: arXiv:2503.11251 source file (2025-03-14)
Supplement: Supplementary file 9 [file self_ref_results_appendix.tex]

% \begin{table*}[t]
% \centering
% \setlength{\tabcolsep}{2pt}
% \caption{\textbf{Self-Reference results on the Mistral-7B.}}
% \label{tab:self-ref-7b-owm}
% \resizebox{\linewidth}{!}{
% \begin{tabular}{l|ccc|cccccccc|c}
% \toprule
% \textbf{Model} & \multicolumn{1}{c}{\textbf{\begin{tabular}[c]{@{}c@{}}SLM\\ Strategy\end{tabular}}} & \multicolumn{1}{c}{\textbf{\begin{tabular}[c]{@{}c@{}}Uniq.\\ Toks$^*$\end{tabular}}}& \multicolumn{1}{c|}{\textbf{\begin{tabular}[c]{@{}c@{}}Train\\ Toks\end{tabular}}} & \textbf{GSM8K} & \textbf{MATH} & \textbf{SVAMP} & \textbf{ASDiv} & \textbf{MAWPS} & \textbf{TAB}& \textbf{MQA} & \multicolumn{1}{c|}{\textbf{\begin{tabular}[c]{@{}c@{}}MMLU\\ STEM\end{tabular}}} & \textbf{AVG} \\
% \midrule
% Mistral-CT (RM) & - & 14B & 15B & 42.9 & 22.2 & 68.6 & 71.0 & 86.1 & 45.1 & 47.7 & 52.6 & 54.5 \\
% Mistral-SLM & $\mathcal{L}_{\text{RM}}(x_i)$ & 14B & 13.5B & 45.1 & 21.0 & 67.4 & 71.6 & 87.0 & 45.2 & 48.9 & 53.3 & 54.9 \\
% Mistral-SLM & $\mathcal{H}_{\text{RM}}(x_i)$ & 14B & 13.5B & 47.7 & 22.8 & 67.8 & 72.0 & 87.7 & 54.4 & 50.5 & 52.8 & 57.0 \\
% \bottomrule
% \end{tabular}
% }
% \end{table*}

\begin{table*}[t]
\centering
\small
\setlength{\tabcolsep}{2pt}
\caption{\textbf{Full Self-Reference results on Tinyllama-1.1B.}}
\label{tab:self-ref-1b-slm}
\resizebox{\linewidth}{!}{
\begin{tabular}{c|c|cccccc|c}
\toprule
\multicolumn{1}{c|}{\textbf{\begin{tabular}[c]{@{}c@{}}Score\\ Function\end{tabular}}} & \multicolumn{1}{c|}{\textbf{\begin{tabular}[c]{@{}c@{}}Select\\ Ratio\end{tabular}}} & \textbf{GSM8K} & \textbf{MATH} & \textbf{SVAMP} & \textbf{ASDiv} & \textbf{MAWPS} & \textbf{MQA} & \textbf{AVG} \\
\midrule
- & 100\% & 6.3 & 2.6 & 21.7 & 36.7 & 47.7 & 13.9 & 21.5 \\
\midrule
\multirow{5}{*}{$\mathcal{L}_{\text{RM}}(x_i)$} & 90\% & \textbf{7.4} & 4.4 & \textbf{23.4} & 38.7 & 51.9 & \textbf{14.4} & 23.4 \\
& 80\% & 6.4 & \textbf{4.6} & 23.1 & 39.7 & 52.0 & 14.3 & 23.4 \\
& 70\% & 6.7 & \textbf{4.6} & 23.3 & \textbf{40.0} & \textbf{54.5} & 14.3 & \textbf{23.9} \\
& 60\% & 7.0 & \textbf{4.6} & 22.2 & 38.5 & 52.2 & 13.7 & 23.0 \\
& 50\% & 5.7 & 4.2 & 20.7 & 36.7 & 46.7 & 10.3 & 20.7  \\
\midrule

\multirow{5}{*}{$\mathcal{H}_{\text{RM}}(x_i)$}
& 90\% & 6.7 & 3.0 & 23.7 & 40.3 & 52.3 & 13.1 & 23.2 \\
& 80\% & 6.8 & 3.6 & 22.5 & \textbf{40.6} & \textbf{52.9} & 13.6 & 23.3 \\
& 70\% & \textbf{7.0} & 4.8 & 23.0 & 39.3 & 50.5 & 13.5 & 23.0 \\
& 60\% & 6.5 & 4.8 & \textbf{26.5} & 37.3 & 49.7 & \textbf{15.6} & \textbf{23.4} \\
& 50\% & 4.7 & \textbf{5.8} & 20.9 & 33.8 & 42.5 & 11.1 & 19.8  \\
\midrule

\multirow{5}{*}{$\mathcal{H}_{\text{RM}}(x_i)\cup\mathcal{L}_{\text{RM}}(x_i)$}
& $50\% \cup 70\% (80\%)$& 6.4 & 3.6 & 22.7 & 38.4 & 52.6 & 15.3 & 23.2 \\
& $70\% \cup 60\% (77\%)$& 6.3 & 4.6 & 24.4 & 39.6 & 51.4 & \textbf{16.3} & \textbf{23.8} \\
& $70\% \cup 50\% (75\%)$& 6.9 & 5.6 & 23.2 & \textbf{39.9} & \textbf{52.9} & 12.6 & 23.5 \\
& $60\% \cup 60\% (70\%)$& 6.7 & 5.2 & \textbf{24.7} & 39.2 & 50.6 & 14.6 & 23.5 \\
& $60\% \cup 50\% (68\%)$& 7.1 & 5.8 & 21.7 & 37.3 & 49.6 & 15.3 & 22.8 \\
& $60\% \cup 40\% (65\%)$& \textbf{7.3} & \textbf{6.0} & 23.6 & 36.9 & 48.6 & 13.1 & 22.6 \\
\midrule

\multirow{5}{*}{$\mathcal{H}_{\text{RM}}(x_i)\cap\mathcal{L}_{\text{RM}}(x_i)$} 
& $80\% \cap 90\% (76\%)$& 6.0 & 4.4 & 23.7 & 38.5 & 51.2 & 13.3 & 22.8 \\
& $75\% \cap 75\% (72\%)$& 7.8 & 5.2 & \textbf{24.2} & 39.4 & \textbf{54.9} & 14.7 & 24.4 \\
& $70\% \cap 90\% (68\%)$& 6.8 & 4.6 & 22.2 & 40.3 & 53.0 & 14.8 & 23.6 \\
& $80\% \cap 80\% (67\%)$& \textbf{8.2} & \textbf{6.4} & 21.2 & 39.1 & 53.4 & 15.0 & 23.9 \\
& $70\% \cap 70\% (60\%)$& 7.1 & 5.0 & 23.5 & \textbf{41.2} & 53.8 & \textbf{18.0} & \textbf{24.8} \\
\bottomrule
\end{tabular}
}
\end{table*}
